# Supplementary material for: Training Automated Defense Strategies Using Graph-based Cyber Attack Simulations
Source: arXiv:2304.11084 source file (2023-04-17)
Supplement: Supplementary file 1 [file appendices.tex]

\appendix

\section{Hyperparameters}\label{hyperparameters}

\begin{table}[!htpb]
	\caption{Hyperparameters used for \ac{PPO} algorithm and policy model.}\label{tab:hyperparameters}
	\centering

\begin{tabular}{lc}
		\textbf{Hyperparameter} & \textbf{Value} \\
 \toprule
		\(k_{vf}\) & 1E-3 \\
		\(k_s\) & 0 \\
		\(k_{kl}\) & 1.0 \\
		Train batch size & 2046 \\
        SGD minibatch size & 256 \\
        VF clip parameter & 500 \\
        Policy loss clip parameter & 0.02 \\
        SGD learning rate & 1E-4 \\
		MLP hidden layers & 2 \\
		MLP hidden layer dim. & 128 \\

\end{tabular}
\end{table}
